# Supplementary material for: Making the Best of Both Worlds: A Domain-Oriented Transformer for Unsupervised Domain Adaptation
Source: arXiv:2208.01195 source file (2022-08-02)
Supplement: Supplementary file 1 [file appendix.tex]

% \section*{Supplementary Material for Paper ID 1983}
In the supplementary we include the following: complete training procedure for our proposed DOT (section~\ref{sec:alg}), proof for the inequalities of our proposed contrastive alignment loss (section~\ref{sec:proof}), detailed introduction to the datasets and augmentations used in our experiment, (section~\ref{sec:dataset}), full table of experiment results on DomainNet (section~\ref{sec:domainnet}), detailed results of the analytical experiments (section~\ref{sec:comparison}), and our results in multi-target domain adaptation setting (section~\ref{sec:mtda}).

\section{Algorithms of Domain-Oriented Transformer}\label{sec:alg}
The complete training procedure for our proposed DOT is shown in Algorithm~\ref{alg:Framwork}. In stage 1, we train a source model using the source supervised loss $\mathcal{L}_s^{sup}$ only to obtain the initial target pseudo-labels. In stage 2, we train a new model with two class tokens from the ImageNet-1k pretrained model. This model is optimized using full objectives introduced in the paper. After certain rounds of training, the target pseudo-labels are updated according to the proposed strategy. The training process continues until the model converges or the max iteration is reached.

\begin{algorithm}[!htbp]
  \small
  \caption{\small Training Algorithm of Domain-Oriented Transformer}
  \label{alg:Framwork}
  \begin{algorithmic} [1]
    \REQUIRE
      Source domain $\{\left(\x_{s}^i,y_{s}^i\right)\}_{i=1}^{n_s}$; Target domain $\{\x_{t}^j\}_{j=1}^{n_t}$; Hyper-parameters $\lambda$, $\beta$ and $\tau$; Metric function $\delta(\cdot)$; Max iteration: $I$
    \ENSURE
      Trained model for target domain: $h_t(f_t(\cdot))$
    \begin{enumerate}
        \item[\textbf{Stage 1}] Obtain Initial Target Pseudo-labels:
    \end{enumerate}
        \STATE Initialize the ViT with parameters pretrained on ImageNet-1k;
        \STATE Train ViT in source domain using $\mathcal{L}_s^{sup}$ as Eq.~(2) in the paper;
        \STATE Obtain the initial target pseudo-labels $\hat{y}^*_{t,1}$ by label refinement;
    \begin{enumerate}
        \item[\textbf{Stage 2}] Knowledge Exploration and Transfer:
    \end{enumerate}
        \STATE Reinitialize the ViT and randomly initialize two classifiers;
        \FOR{$i=1,2,\cdots,I$}
            \STATE Obtain $f_s(\x_{s}), \; f_t(\x_{s}), \; f_s(\x_{t}), \; f_t(\x_t)$;
            \STATE Compute $\mathcal{L}^{sup}$ by Eq.~(4) with source labels $y_{s}$ and current target pseudo-labels $\hat{y}^*_{t,i}$;
            \STATE Normalize the features to $\tilde{f}_s(\x_{s}), \; \tilde{f}_t(\x_{s}), \; \tilde{f}_s(\x_{t}), \; \tilde{f}_t(\x_t)$;
            \STATE Calculate $\mathcal{L}^{con}$ by Eq.~(7) and $\mathcal{L}^{diff}$ by Eq.~(10) in the paper;
            % \STATE Using $\textbf{g}^s_{si},\textbf{f}^s$ to calculate $L_s$ and $L_s^{con}$;
            % \STATE Using $\textbf{g}^t_{tj} , \textbf{t}^t$ to calculate $L_t$ and $L_t^{con}$;
            \STATE Accumulate the above losses and back propagate;
            \STATE Obtain new pseudo-labels $\hat{y}^*_{t,i+1}$ using label refinement strategy with metric $\delta(\cdot)$.
        \ENDFOR
  \end{algorithmic}
\end{algorithm}

\section{Proof of the inequalities}\label{sec:proof}
In this section, we show why minimizing the domain-oriented contrastive loss maximizes the domain-specific information. The proof for the two inequalities are similar since they are symmetric, hence we only need to prove one of them. Here we prove the inequality of target-oriented contrastive loss.

We start by considering a simplified but equivalent situation, where there is only one positive target sample for each source. Formally, the target-oriented features for source and target samples are represented as $f_t^{si} = f_t(\x_s^i),f_t^{tj} = f_t(\x_t^j)$ and the normalized feature are $\tilde{f}_t^{si},\tilde{f}_t^{tj}$ respectively.
For each source sample $\tilde{f}^{si}$ as query, the key set $\boldsymbol{T}=\{\tilde{f}^{t1},...,\tilde{f}^{tN}\}$ consists of one corresponding positive target sample $\tilde{f}^{t+}$ and $N-1$ negatives. To simplify our notation, we omit the subscript $t$ for denoting the features to be target-oriented and use $\tilde{f}^{si},\tilde{f}^{tj}$ instead in the following proof. Then, the expectation of $\mathcal{L}_{t}^{con}$ can be written as
\begin{equation}
	\mathbb{E} [\mathcal{L}_t^{con}] = \mathbb{E}_{\tilde{f}^s,\boldsymbol{T}} \left[ -\log \frac{{\rm exp}(\tilde{f}^{s\top} \tilde{f}^{t+} /\tau)}{\sum_{j=1}^{N} {\rm exp}(\tilde{f}^{s\top} \tilde{f}^{tj} /\tau)}\right].
\end{equation}

Assume query $\tilde{f}^{si}$ has the label $y$, then the positive sample $\tilde{f}^{t+}$ can be regarded as drawn from distribution $p(\tilde{f}^t|\tilde{f}^{si},y)$, while the negative samples are drawn from $p(\tilde{f}^t)$. Therefore, the optimal possibility that the target sample $\tilde{f}^{tj}$ is positive can be derived as
\begin{equation}
	P^{pos}(\tilde{f}^{tj}|\boldsymbol{T})=\frac{p(\tilde{f}^{tj}|\tilde{f}^{si},y)\prod_{l\neq j}p(\tilde{f}^{tl})}{\sum_{k=1}^N p(\tilde{f}^{tk}|\tilde{f}^{si},y)\prod_{l\neq k}p(\tilde{f}^{tl})}=\frac{\frac{p(\tilde{f}^{tj}|\tilde{f}^{si},y)}{p(\tilde{f}^{tj})}}{\sum_{k=1}^N \frac{p(\tilde{f}^{tk}|\tilde{f}^{si},y)}{p(\tilde{f}^{tk})}},
\end{equation}
which indicates that the optimal value for ${\rm exp}(\tilde{f}^{si\top} \tilde{f}^{t+} /\tau)$ is $\frac{p(\tilde{f}^{t+}|\tilde{f}^s,y)}{p(\tilde{f}^{t+})}$. Thus, we have
\begin{align}
	\mathbb{E}[\mathcal{L}_t^{con}] &\geq \mathbb{E}[\mathcal{L}_t^{con,\rm optimal}]\\ &= \mathop{\mathbb{E}}\limits_{\tilde{f}^s,y,\boldsymbol{T}}\left[ -\log \frac{\frac{p(\tilde{f}^{t+}|\tilde{f}^s,y)}{p(\tilde{f}^{t+})}}{\sum_{k=1}^N \frac{\tilde{f}^{tk}|p(\tilde{f}^s,y)}{p(\tilde{f}^{tk})}} \right] \\
	&= \mathop{\mathbb{E}}\limits_{\tilde{f}^s,y,\boldsymbol{T}} \left[ -\log \frac{\frac{p(\tilde{f}^{t+}|\tilde{f}^s,y)}{p(\tilde{f}^{t+})}}{\frac{p(\tilde{f}^{t+}|\tilde{f}^s,y)}{p(\tilde{f}^{t+})} + \sum_{\tilde{f}^{tj} \neq \tilde{f}^{t+}} \frac{p(\tilde{f}^{tj}|\tilde{f}^s,y)}{p(\tilde{f}^{tj})}} \right] \\
	&= \mathop{\mathbb{E}}\limits_{\tilde{f}^s,y,\boldsymbol{T}}  \log \left[  1+ \frac{p(\tilde{f}^{t+})}{p(\tilde{f}^{t+}|\tilde{f}^s,y)}\sum_{\tilde{f}^{tj} \neq \tilde{f}^{t+}} \frac{p(\tilde{f}^{tj}|\tilde{f}^s,y)}{p(\tilde{f}^{tj})} \right] \\
	&\approx \mathop{\mathbb{E}}\limits_{\tilde{f}^s,y,\boldsymbol{T}}  \log \left[  1+ \frac{p(\tilde{f}^{t+})}{p(\tilde{f}^{t+}|\tilde{f}^s,y)} \left((N-1)\mathop{\mathbb{E}}\limits_{\tilde{f}^t} \frac{p(\tilde{f}^{tj}|\tilde{f}^s,y)}{p(\tilde{f}^{tj})}\right) \right] \\
	&=\mathop{\mathbb{E}}\limits_{\tilde{f}^s,y,\boldsymbol{T}} \log \left[ 1+\frac{p(\tilde{f}^{t+})}{p(\tilde{f}^{t+}|\tilde{f}^s,y)}(N-1) \right] \\
	&\geq \mathop{\mathbb{E}}\limits_{\tilde{f}^s,y,\boldsymbol{T}} \log \left[\frac{p(\tilde{f}^{t+})}{p(\tilde{f}^{t+}|\tilde{f}^s,y)}(N-1)\right] \\
	&=-I(\tilde{f}^t;\tilde{f}^s,y) + \log (N-1) \\
  &\geq -I(f^t;f^s,y)+ \log (N-1).
\end{align}
The last step follows the data processing inequality, and we can further split the information $I(f^t;f^s,y)$ to $I(f^t;f^s)+I(f^t;y|f^s)$ using the chain rule of mutual information. The first term refers to the mutual information of source and target samples in the target-oriented feature space and the second term is the task-relevant information for target domain that is independent of source domain.
Thus, minimizing the target-oriented contrastive loss simultaneously improves domain alignment and target-specific information exploration. Following similar derivation, we can obtain the corresponding conclusion for source-oriented contrastive loss.

% \section{Conflict between perfect domain alignment and superior classification performance}
% We give an argument showing that under certain conditions, one cannot simultaneously achieve perfect domain alignment in a common feature space and superior classification performance. Therefore, learning two domain-oriented feature spaces such that each one guarantees the classification performance in one domain is more appropriate when such conflict exits. The argument follows~\cite{liu2021adversarial}.

% The goal for perfect marginal probability alignment in one feature space is $P_s(f(\x))=P_t(f(\x))$, which can be written as:
% \begin{equation}
% 	\sum_{k=1}^K P_s(f(\x)|y=k)P_s(y=k) = \sum_{k=1}^K P_t(f(\x)|y=k)P_t(y=k).
% \end{equation}
% In order to achieve superior classification performance, features for each class must be totally distinguishable, which means that for each sample $\x$ with true label $\hat{y}$, we have
% \begin{equation}
% 	P_s(f(\x)|y=\hat{y})>0 \ \text{and} \ P_s(f(\x)|y\neq \hat{y})=0;
% \end{equation}
% as well as
% \begin{equation}
% 	P_t(f(\x)|y=\hat{y})>0 \ \text{and} \ P_t(f(\x)|y\neq \hat{y})=0.
% \end{equation}
% Therefore, the perfect alignment actually requires
% \begin{equation}
% 	P_s(f(\x)|y=\hat{y})P_s(y=\hat{y}) = P_t(f(\x)|y=\hat{y})P_t(y=\hat{y});
% \end{equation}
% By taking the integral over all samples that have a same class

\section{Experimental details}\label{sec:dataset}
We first introduce with more details the three benchmarks that is used in our experiment: Office-Home~\cite{Office-Home}, VisDA-2017~\cite{VisDA2017} and DomainNet~\cite{DomainNet}. Then we introduce the augmentations used in training. 

\textbf{Office-Home} is a standard dataset for DA which contains four different domains: Artistic(\textbf{Ar}), Clip Art(\textbf{Cl}), Product(\textbf{Pr}) and Real-world(\textbf{Re}). Each domain consists of 65 object categories found typically in office and home scenarios.

\textbf{VisDA-2017} is a 12-class UDA classification dataset for cross-domain tasks from synthetic(\textbf{S}) to real(\textbf{R}). Among them, the training set incorporates 152,397 synthetic images and the validation set contains 55,388 real-world images collected from Microsoft COCO~\cite{Microsoft2014}. %In our experiments, we denote training set as \textbf{S} and validation set as \textbf{R}, and construct one transfer task: \textbf{S}$\rightarrow$\textbf{R}.

\textbf{DomainNet} is currently the largest and the most challenging cross-domain benchmark. The whole dataset comprises $\sim$0.6 million images drawn from 345 categories and six diverse domains: Infograph(\textbf{inf}), Quickdraw(\textbf{qdr}), Real(\textbf{rel}), Sketch(\textbf{skt}), Clipart(\textbf{clp}), Painting(\textbf{pnt}). Thirty adaptation tasks can be constructed to evaluate UDA methods, i.e., \textbf{inf$\rightarrow$qdr}, ..., \textbf{pnt$\rightarrow$clp}.
%In particular, there are significantly different visual patterns across domains, which can be real-world images or abstract creations.

In the training procedure, we adopt the data-augmentation techniques Rand-Augment~\cite{randaugment} and random erasing~\cite{random_erase} to fully utilize the limited training data and improve the model's generalization ability follows DeiT~\cite{DeiT}. We find these data-augmentations very helpful for training Transformers in UDA tasks.

\section{Complete Experimental Results on DomainNet Dataset}\label{sec:domainnet}
We present the complete results of on DomainNet, including DOT-S and DOT-B, and baselines of both CNN-based methods and ViT-based methods. The results are shown in Table~\ref{tab:domainnetbase} in the next page. We can conclude that DOT achieves superior performance on DomainNet benchmark, reaching an average accuracy of 43.4\% using DOT-B which is 9.3\% higher than its backbone ViT-B. Also, we observe that DOT-S already outperforms CDTrans-B by an average of 4.2\% as well as all the UDA methods that are based on ResNet-50 backbone. These results validate the effectiveness of our method, proving that training the target-oriented feature spaces and an individual target classifier using only target data and pseudo-labels is applicable when using Transformer as backbone. 

\section{Complete results of analytical experiments}\label{sec:comparison}
In the analysis, we compare different variants of our method to empirically validate the effectiveness of our contrastive-based alignment loss, our pseudo-label refinement strategy as well as our choice of the metric function. Due to limited space, we only present the average results of each experiment. Here we show the full results of the comparisons in Table~\ref{tab:align_supp},~\ref{tab:pseudo-labeling_supp},~\ref{tab:metric_supp}.

\begin{table}[htbp]
  \centering
  \caption{Multi-target domain adaptation on Office-Home.}
  \vspace{-8pt}
  \resizebox{0.45\textwidth}{!}{
   \begin{tabular}{l|cccc>{\columncolor{lightgray}}c}
  \specialrule{.1em}{.05em}{.05em}
   Method & \textbf{Ar} $\rightarrow$ Cl,Pr,Re & \textbf{Cl} $\rightarrow$ Ar,Pr,Re& \textbf{Pr} $\rightarrow$ Ar,Cl,Re & \textbf{Re} $\rightarrow$ Ar,Cl,Pr & Avg.\\
   \hline
   ResNet-50~\cite{resnet} & 47.6 & 42.6 & 44.2 & 51.3 & 46.4 \\
   + MT-MTDA~\cite{hgan} & 64.6 & 66.4 & 59.2 & 67.1 & 64.3 \\
   + D-CGCT~\cite{dcgct} & 70.5 & 71.6 & 66.0  & 71.2 & 69.8 \\
   \hline
   ViT-S~\cite{vit} & 69.3 & 72.7 & 64.6 & 69.7 & 69.1 \\
   + \textbf{DOT-S} (\textit{ours}) & \textbf{75.4} & \textbf{80.3} & \textbf{71.6} & \textbf{73.9} & \textbf{75.3} \\
   \specialrule{.1em}{.05em}{.05em}
   \end{tabular}}
  \label{tab:multi-target}%
\end{table}%

\section{Extension on Multi-target domain adaptation}\label{sec:mtda}
In addition to the extension of our method to multi-source domain adaptation, we show that DOT can also be extended to multi-target domain adaptation (MTDA) scenario, where a single model is required to adapt to multiple target domains. As shown in Table~\ref{tab:multi-target}, each column represents the average accuracy on three target domains. We observe that DOT-S outperforms CNN-based MTDA approaches significantly. 

\begin{table*}[htbp]
  \centering
  \caption{Complete table of accuracy (\%) results on DomainNet for unsupervised domain adaption. In each sub-table, the column-wise domains are selected as the source domain and the row-wise domains are selected as the target domain. Methods from the first two rows are based on ResNet-50 backbone, while the methods from the last two rows are based on ViT-Small/Base architectures.}
  \vspace{-8pt} 
   \resizebox{\textwidth}{!}{
  \setlength{\tabcolsep}{0.5mm}{
    \begin{tabular}{|c|ccccccc|c|ccccccc||c|ccccccc|c|ccccccc|}
    \specialrule{.1em}{.05em}{.05em}
    {ResNet50\cite{resnet}} & {  clp}   & {  inf}   & {  pnt}   & {  qdr}   & {  rel}   & {  skt}   & Avg.  & 
    {MCD\cite{MCD}} & {  clp}   & {  inf}   & {  pnt}   & {  qdr}   & {  rel}   & {  skt}   & Avg.  & 
    {CDAN\cite{CDAN}} & {  clp}   & {  inf}   & {  pnt}   & {  qdr}   & {  rel}   & {  skt}   & Avg.  \\
    \hline
    {  clp}   & --    & 14.2  & 29.6  & 9.5   & 43.8  & 34.3  & 26.3  & {  clp}   & --    & 15.4  & 25.5  & 3.3   & 44.6  & 31.2  & 24.0  & {  clp}   & --    & 13.5  & 28.3  & 9.3   & 43.8  & 30.2  & 25.0 \\
    {  inf}   & 21.8  & --    & 23.2  & 2.3   & 40.6  & 20.8  & 21.7  & {  inf}   & 24.1  & --    & 24.0  & 1.6   & 35.2  & 19.7  & 20.9  & {  inf}   & 16.9  & --    & 21.4  & 1.9   & 36.3  & 21.3  & 20.0 \\
    {  pnt}   & 24.1  & 15.0  & --    & 4.6   & 45.0  & 29.0  & 23.5  & {  pnt}   & 31.1  & 14.8  & --    & 1.7   & 48.1  & 22.8  & 23.7  & {  pnt}   & 29.6  & 14.4  & --    & 4.1   & 45.2  & 27.4  & 24.2 \\
    {  qdr}   & 12.2   & 1.5  & 4.9   & --    & 5.6   & 5.7   & 6.0   & {  qdr}   & 8.5   & 2.1   & 4.6   & --    & 7.9   & 7.1   & 6.0   & {  qdr}   & 11.8  & 1.2   & 4.0   & --    & 9.4   & 9.5   & 7.2  \\
    {  rel}   & 32.1  & 17.0  & 36.7  & 3.6   & --    & 26.2  & 23.1  & {  rel}   & 39.4  & 17.8  & 41.2  & 1.5   & --    & 25.2  & 25.0  & {  rel}   & 36.4  & 18.3  & 40.9  & 3.4   & --    & 24.6  & 24.7 \\
    {  skt}   & 30.4  & 11.3  & 27.8  & 3.4   & 32.9  & --    & 21.2  & {  skt}   & 37.3  & 12.6  & 27.2  & 4.1   & 34.5  & --    & 23.1  & {  skt}   & 38.2  & 14.7  & 33.9  & 7.0   & 36.6  & --    & 26.1 \\
    Avg.      & 24.1  & 11.8  & 24.4  & 4.7   & 33.6  & 23.2  & \cellcolor{lightgray}{20.3}  & Avg.      & 28.1  & 12.5  & 24.5  & 2.4   & 34.1  & 21.2  & \cellcolor{lightgray}{20.5}  & Avg.      & 27.0  & 12.4  & 25.7  & 5.1   & 34.3  & 22.6  & \cellcolor{lightgray}{21.2} \\
    \specialrule{.1em}{.05em}{.05em}
    \specialrule{.1em}{.05em}{.05em}
    BNM\cite{BNM} & {  clp}   & {  inf}   & {  pnt}   & {  qdr}   & {  rel}   & {  skt}   & Avg.  & 
    BCDM\cite{BCDM} & {  clp}   & {  inf}   & {  pnt}   & {  qdr}   & {  rel}   & {  skt}   & Avg.  &
    SCDA\cite{scda} & {  clp}   & {  inf}   & {  pnt}   & {  qdr}   & {  rel}   & {  skt}   & Avg. \\
    \hline
    {  clp}   & --    & 12.1  & 33.1  & 6.2  & 50.8  & 40.2  & 28.5  & {  clp}   & --    & 17.2  & 35.2  & 10.6  & 50.1  & 40.0  & 30.6 & {  clp}   & --     & 18.6  & 39.3  & 5.1   & 55.0  & 44.1  & 32.4 \\
    {  inf}   & 26.6  & --    & 28.5  & 2.4  & 38.5  & 18.1  & 22.8  & {  inf}   & 29.3  & --    & 29.4  & 3.8   & 41.3  & 25.0  & 25.8 & {  inf}   & 29.6   & --    & 34.0  & 1.4   & 46.3  & 25.4  & 27.3 \\
    {  pnt}   & 39.9  & 12.2  & --    & 3.4  & 54.5  & 36.2  & 29.2  & {  pnt}   & 39.2  & 17.7  & --    & 4.8   & 51.2  & 34.9  & 29.6 & {  pnt}   & 44.1   & 19.0  & --    & 2.6   & 56.2  & 42.0  & 32.8 \\
    {  qdr}   & 17.8  & 1.0   & 3.6   & --   & 9.2   & 8.3   & 8.0   & {  qdr}   & 19.4  & 2.6   & 7.2   & --    & 13.6  & 12.8  & 11.1 & {  qdr}   & 30.0   & 4.9   & 15.0  & --    & 25.4  & 19.8  & 19.0 \\
    {  rel}   & 48.6  & 13.2  & 49.7  & 3.6  & --    & 33.9  & 29.8  & {  rel}   & 48.2  & 21.5  & 48.3  & 5.4   & --    & 36.7  & 32.0 & {  rel}   & 54.0   & 22.5  & 51.9  & 2.3   & --    & 42.5  & 34.6 \\
    {  skt}   & 54.9  & 12.8  & 42.3  & 5.4  & 51.3  & --    & 33.3  & {  skt}   & 50.6  & 17.3  & 41.9  & 10.6  & 49.0  & --    & 33.9 & {  skt}   & 55.6   & 18.5  & 44.7  & 6.4   & 53.2    & --  & 35.7 \\
    Avg.      & 37.6  & 10.3  & 31.4  & 4.2  & 40.9  & 27.3  & \cellcolor{lightgray}{25.3}  & Avg.      & 37.3  & 15.3  & 32.4  & 7.0   & 41.0  & 29.9  & \cellcolor{lightgray}{27.2} & Avg.      & 37.6   & 14.6  & 31.5  & 14.8  & 43.3  & 28.8  & \cellcolor{lightgray}{28.4} \\
    \specialrule{.1em}{.05em}{.05em}
    \specialrule{.1em}{.05em}{.05em}
    ViT-S~\cite{vit} & {  clp}   & {  inf}   & {  pnt}   & {  qdr}   & {  rel}   & {  skt}   & Avg.  &
    CDTrans-S~\cite{cdtrans} & {  clp}   & {  inf}   & {  pnt}   & {  qdr}   & {  rel}   & {  skt}   & Avg.  & 
    \textbf{DOT-S} & {  clp}   & {  inf}   & {  pnt}   & {  qdr}   & {  rel}   & {  skt}   & Avg. \\
    \hline
    {  clp}  &  --   & 19.3  & 43.2  & 14.3  & 58.8  & 46.4  & 36.4  &  {  clp}  & --    & 24.2  & 47.0  & 22.3  & 64.3  & 50.6  & 41.7  &  {  clp}  & --    & 19.5 &  51.3 &  27.5 &  67.6 &  51.7 &  43.5 \\
    {  inf}  & 35.2  &  --   & 36.7  & 4.7   & 50.4  & 30.0  & 31.4  &  {  inf}  & 45.3  & --    & 45.3  & 6.6   & 62.8  & 38.3  & 39.7  &  {  inf}  & 59.5 & -- &  51.5 &  14.2 &  69.9 &  46.8 &  48.4  \\
    {  pnt}  & 44.7  & 18.7  &  --   & 4.5   & 59.0  & 38.1  & 33.0  &  {  pnt}  & 53.6  & 20.4  & --    & 10.6  & 63.9  & 42.4  & 38.2  &  {  pnt}  & 58.5 &  18.9 & -- &  16.5 &  70.4 &  47.2 &  42.3 \\
    {  qdr}  & 23.2  & 3.3   & 10.1  &  --   & 17.0  & 14.5  & 13.6  &  {  qdr}  & 2.8   & 0.2   & 0.6   & --    & 0.7   & 4.2   & 1.7   &  {  qdr}  & 39.3 &  6.1 &  22.3 & -- &  34.7 &  25.6 &  25.6 \\
    {  rel}  & 48.3  & 18.9  & 50.4  & 7.0   &  --   & 37.0  & 32.3  &  {  rel}  & 47.1  & 17.9  & 45.0  & 7.9   & --    & 31.7  & 29.9  &  {  rel}  & 62.3 &  20.0 &  57.0 &  20.9 & -- &  49.4 &  41.9 \\
    {  skt}  & 54.3  & 16.5  & 41.1  & 15.3  & 53.8  &  --   & 36.2  &  {  skt}  & 61.0  & 19.3  & 46.8  & 22.8  & 59.2  & --    & 41.8  &  {  skt}  & 64.6 &  16.8 &  49.9 &  30.4 &  65.4 & -- &  45.4   \\
    Avg.     & 41.1  & 15.3  & 36.3  & 9.2   & 47.8  & 33.2  & \cellcolor{lightgray}{30.5}  &  Avg.     & 42.0  & 16.4  & 36.9  & 14.0  & 50.2  & 33.4  & \cellcolor{lightgray}{32.2}  &  Avg.     & 56.8 &  16.3 &  46.4 &  21.9 &  61.6 &  44.1 & \cellcolor{lightgray}{\textbf{41.2}} \\
    \specialrule{.1em}{.05em}{.05em}
    \specialrule{.1em}{.05em}{.05em}     ViT-B\cite{vit} & {  clp}   & {  inf}   & {  pnt}   & {  qdr}   & {  rel}   & {  skt}   & Avg.  &     CDTrans-B\cite{cdtrans} & {  clp}   & {  inf}   & {  pnt}   & {  qdr}   & {  rel}   & {  skt}   & Avg.  &     \textbf{DOT-B} & {  clp}   & {  inf}   & {  pnt}   & {  qdr}   & {  rel}   & {  skt}   & Avg. \\     \hline     {  clp}  &   --    & 20.1  & 46.2  & 13.0  & 62.3  & 48.8  & 38.1 & {  clp}  & --    & 27.9  & 57.6  & 27.9  & 73.0  & 58.8  & 49.0  &  {  clp}  & --    & 20.2  & 53.6  & 26.7  & 71.2  & 55.2  & 45.4  \\     {  inf}  &   46.4  & --    & 45.2  & 5.1   & 62.3  & 37.5  & 39.3 & {  inf}  & 58.6  & --    & 53.4  & 9.6   & 71.1  & 47.6  & 48.1  &  {  inf}  & 63.0 &  --   & 54.6  & 12.3  & 73.1  & 50.7  & 50.7    \\     {  pnt}  &   48.1  & 19.1  & --    & 4.4   & 62.5  & 41.8  & 35.2 & {  pnt}  & 60.7  & 24.0  & --    & 13.0  & 69.8  & 49.6  & 43.4  &  {  pnt}  & 61.8  & 20.3   & --    & 11.4  & 72.2  & 50.5  & 43.2  \\     {  qdr}  &   28.2  & 5.2   & 14.4  & --    & 21.9  & 17.7  & 17.5 & {  qdr}  & 2.9   & 0.4   & 0.3   & --    & 0.7   & 4.7   & 1.8  &  {  qdr}  & 47.3  & 7.4  & 30.3   &  --   & 44.6  & 33.7  & 32.7    \\     {  rel}  &   53.2  & 19.3  & 53.5  & 7.2   & --    & 41.6  & 35.0 & {  rel}  & 49.3  & 18.7  & 47.8  & 9.4   & --    & 33.5  & 31.7  &  {  rel}  & 62.9  & 20.0  & 56.9  & 17.3    & --    & 49.3  & 41.3  \\     {  skt}  &   58.0  & 18.5  & 46.5  & 15.7  & 58.7  & --    & 39.5 & {  skt}  & 66.8  & 23.7  & 54.6  & 27.5  & 68.0  & --    & 48.1  &  {  skt}  & 67.3  & 18.7  & 52.9  & 27.8  & 69.8   & --    &  47.3  \\     Avg.     &   46.8  & 16.4  & 41.2  & 9.1   & 53.5  & 37.5  & \cellcolor{lightgray}{34.1} &  Avg.    & 47.7  & 18.9  & 42.7  & 17.5  & 56.5  & 38.8  & \cellcolor{lightgray}{37.0}  &  Avg.     & 60.5  & 17.3  & 49.7  & 19.1  & 66.2  & 47.9  & \cellcolor{lightgray}{\textbf{43.4}}  \\     \specialrule{.1em}{.05em}{.05em}
    \end{tabular}%
    \label{tab:domainnetbase} }}%
    \vspace{5pt}
\end{table*}%

\begin{table*}[htbp]
  \centering
  \caption{Full results of the comparison between alignment variants on Office-Home.}
  \vspace{-8pt}
  \resizebox{0.98\textwidth}{!}{
   \begin{tabular}{c|lcccccccccccc>{\columncolor{lightgray}}c}
    \specialrule{.1em}{.05em}{.05em}
   Variant & Method& Ar$\rightarrow$Cl & Ar$\rightarrow$Pr & Ar$\rightarrow$Re & Cl$\rightarrow$Ar & Cl$\rightarrow$Pr & Cl$\rightarrow$Re & Pr$\rightarrow$Ar & Pr$\rightarrow$Cl &Pr$\rightarrow$Re & Re$\rightarrow$Ar & Re$\rightarrow$Cl & Re$\rightarrow$Pr & Avg. \\
   \hline
   \multirow{4}{*}{\begin{tabular}[c]{@{}c@{}}Alignment\\ Methods\end{tabular}}
   &w/ MDD~\cite{MDD} & 60.8 &	81.3 &	83.9 &	72.3 &	82.4 &	82.7 &	71.6 &	58.7 &	84.8 &	76.5&	61.1 &	86.4 &	75.2 \\

   &w/ DANN~\cite{DANN}& 61.4 &	81.2 &	83.9 &	73.3 &	81.2 &	83.5 	&69.6 &	56.4 &	84.8& 	77.3 &	60.9 &	85.7& 	74.9   \\
   &w/ TCL~\cite{TCL}&  63.3  &	82.0& 	83.8 	&74.2 	&83.5 &	\textbf{84.2} &	72.3 &	\textbf{61.7} &	\textbf{85.0} &	76.0 &	63.6 &	86.6 &	76.3 \\
   &w/ \textit{\textbf{ours}}& \textbf{63.7}& 	\textbf{82.2}& 	\textbf{84.3}& 	\textbf{74.9}& 	\textbf{84.3} & 	83.0& 	\textbf{72.4}& 	61.0& 	84.8& 	\textbf{76.4}& 	\textbf{64.1}& 	\textbf{86.7} &\textbf{76.5} \\
   \specialrule{.1em}{.05em}{.05em}
   \end{tabular}
  }\label{tab:align_supp}
  \vspace{5pt}
\end{table*}%

\begin{table*}[htbp]
  \centering
  \caption{Full results of the comparison between pseudo-labeling variants on Office-Home.}
  \vspace{-8pt}
  \resizebox{0.98\textwidth}{!}{
   \begin{tabular}{c|lcccccccccccc>{\columncolor{lightgray}}c}
    \specialrule{.1em}{.05em}{.05em}
   Variant & Method& Ar$\rightarrow$Cl & Ar$\rightarrow$Pr & Ar$\rightarrow$Re & Cl$\rightarrow$Ar & Cl$\rightarrow$Pr & Cl$\rightarrow$Re & Pr$\rightarrow$Ar & Pr$\rightarrow$Cl &Pr$\rightarrow$Re & Re$\rightarrow$Ar & Re$\rightarrow$Cl & Re$\rightarrow$Pr & Avg. \\
   \hline
   \multirow{4}{*}{\begin{tabular}[c]{@{}c@{}}Pseudo-labeling\\ Methods\end{tabular}}
   &w/ Confidence & 58.9 &	78.5 &	82.2 &	69.4 &	77.2 &	80.3 &	67.9 &	55.8 &	83.9&	73.5 &	58.6 &	84.9 &72.6\\

   &w/ CBST~\cite{CBST}& 60.7 &	78.4	&82.1 &	72.3&	80.0&	81.5	&69.1&	56.8	&84.9&	74.0	&58.4 &	86.5 &	73.7\\
   &w/ SHOT~\cite{SHOT}&    62.5 &	\textbf{82.2}& 	84.0& 	74.5& 	83.2& 	\textbf{83.5}& 	\textbf{72.4}& 	59.0& 	\textbf{85.1}& 	\textbf{76.8} &	63.1 &	\textbf{87.9}& 	76.2   \\
   &w/ \textit{\textbf{ours}}& \textbf{63.7}& 	\textbf{82.2}& 	\textbf{84.3}& 	\textbf{74.9}& 	\textbf{84.3}& 	83.0& 	\textbf{72.4}& 	\textbf{61.0}& 	84.8& 	76.4& 	\textbf{64.1}& 	86.7 &\textbf{76.5} \\
   \specialrule{.1em}{.05em}{.05em}
   \end{tabular}
  }\label{tab:pseudo-labeling_supp}
  \vspace{5pt}
\end{table*}%

\begin{table*}[htbp]
  \centering
  \caption{Full results of the comparison between metric function variants on Office-Home.}
  \vspace{-8pt}
  \resizebox{0.98\textwidth}{!}{
   \begin{tabular}{c|ccccccccccccc>{\columncolor{lightgray}}c}
    \specialrule{.1em}{.05em}{.05em}
   Variant & Method& Ar$\rightarrow$Cl & Ar$\rightarrow$Pr & Ar$\rightarrow$Re & Cl$\rightarrow$Ar & Cl$\rightarrow$Pr & Cl$\rightarrow$Re & Pr$\rightarrow$Ar & Pr$\rightarrow$Cl &Pr$\rightarrow$Re & Re$\rightarrow$Ar & Re$\rightarrow$Cl & Re$\rightarrow$Pr & Avg. \\
   \hline
   \multirow{3}{*}{\begin{tabular}[c]{@{}c@{}}Metric\\ Function\end{tabular}}
   & \small $\delta_{conf}$& 61.9 &	80.8 &	83.8 &	73.5 &	82.6	&82.3 &	72.3 &	59.5 &	84.2 &	76.0 &	62.2 &	87.0 &	75.5   \\

   & \small $\delta_{ent}$&  62.3 &	80.8 &	83.2 &	73.0 &	82.3 &	82.2 &	71.8 &	60.4 &	84.1 &	75.8	 &61.9 &	\textbf{87.3} &	75.4   \\
   & \small $\delta_{energy}$ & \textbf{63.7}& 	\textbf{82.2}& 	\textbf{84.3}& 	\textbf{74.9}& 	\textbf{84.3}& 	\textbf{83.0}& 	\textbf{72.4}& \textbf{	61.0}& 	\textbf{84.8}& 	\textbf{76.4}& 	\textbf{64.1}& 	86.7 &\textbf{76.5} \\
   \specialrule{.1em}{.05em}{.05em}
   \end{tabular}
  }\label{tab:metric_supp}
\end{table*}%
